# Supplementary material for: Investigations on Speech Recognition Systems for Low-Resource Dialectal Arabic-English Code-Switching Speech
Source: arXiv:2108.12881 source file (2021-08-29)
Supplement: Supplementary file 1 [file appendix.tex]

\section{Appendix}
\label{sec:appendix-morphCS}
We provide a list of the prefixes and suffixes occurring in morphological CS words in ArzEn corpus, along with their frequencies.

\begin{table*}
\begin{adjustbox}{max width=\textwidth}
\begin{tabular}{|l|l|l|r|l|}\hline
\textbf{Affix} & \textbf{Meaning} & \textbf{Frequency} & \textbf{Examples} & \textbf{Translation} \\\hline
\multicolumn{5}{|c|}{\textbf{Proclitics}} \\\hline
\<ال> &  Definite article & 1,995 &WEEKENDS+\<ال> & the weekends \\\hline
\<ف> & 
Conjunction `so/then' & 83 & THEREFORE+\<ف> & so therefore \\\hline
 \<ك> & Preposition `as' & 60 & STUDENT+\<ك> & as (a) student \\\hline
 \<ل> & Preposition `to/for' & 45 & LEVEL+\<ل> & to (a) level \\\hline
 \<ب> & Preposition `with' & 36 &ATTITUDE+\<ب>& with (an) attitude \\\hline
 \<ه> or \<ح> & 
Imperfect future verb & 7 & SUBMIT+\<ه> & will submit \\\hline
\multicolumn{5}{|c|}{\textbf{Enclitics}} \\\hline
\<ه> & 
3rd person possessive pronoun (masc.) & 4 & 
\multicolumn{1}{|l|}{CAREER\#\<ه>}
&his career  \\\hline
\<ها> &
3rd person direct object pronoun (fem.) & 1 & \<ها>\#PROPAGATE+\<ي> & (he) propagates it\\\hline
\<ى> & 
1st person possessive pronoun  & 1 & 
\multicolumn{1}{|l|}{MOBILE\#\<ى>}
& my mobile \\\hline
\multicolumn{5}{|c|}{\textbf{Prefixes}} \\\hline
 \<ا>& 
 1st person imperfect verb (sg.) & 71 & IMPLEMENT+\<ا> & to implement \\\hline
\<ي> & 
3rd person imperfect verb (masc.) & 49 & BREAK+\<ي> & to break \\\hline
 \<ب> & Present tense marker & 46 & USE+\<ب> & to use \\\hline
\<ت> & 
2nd person imperfect verb (masc.) & 33 & PARTICIPATE+\<ت> & to participate \\\cline{2-2}\cline{4-5}
 & 
3rd person imperfect verb (fem.) &  & SUPPORT+\<ت> & to participate \\\hline
\<ن> & 
1st person imperfect verb (pl.) & 14 & DETECT+\<ن> & to detect \\\hline
\<م>& Present participle & 1 & EXPECT+\<م> & EXPECTING \\\hline
\multicolumn{5}{|c|}{\textbf{Suffixes}} \\\hline
\<ات> & Feminine plural & 7 & 
\multicolumn{1}{|l|}{EVENT\#\<ات>}
& events \\\hline
\<نى> & 
1st person direct object pronoun  & 1 & \<نى>\#EVALUATE+\<بي> & he evaluates me\\\hline
\multicolumn{5}{|c|}{\textbf{Circumfixes}} \\\hline
\<وا> + \<ي>& 
3rd person imperfect verb (pl.)  & 4 & \<وا>\#ADAPT+\<ي> & (they) adapt\\\hline
\<ى> + \<ت>& 
2rd person imperfect verb (fem.)  & 2 & \<ى>\#CODE+\<ت> & to code\\\hline
\<وا> + \<ت>&
2rd person imperfect verb (pl.)  & 1 & \<وا>\#PRESENT+\<ت> & to present\\\hline
\multicolumn{5}{|c|}{\textbf{Combinations}} \\\hline
\<بال> & Combination of the morphemes: \<ب> (preposition) and \<ال>
& 85 & Mobile+\<بال> & with the mobile \\\hline
\<لل> & Combination of the morphemes: \<ل> and \<ال> & 36 &LIMIT+\<لل> & to the limit  \\\hline
\<بي> & 
Combination of the morphemes: \<ب> (present tense) and \<ي> & 27 & APPRECIATE+\<بي> & (he/it) appreciates \\\hline
\<بت> & 
Combination of the morphemes: \<ب> (present tense) 
& 19 & OVERCOME+\<بت> & (you) overcome \\
& and \<ت> (2nd person imperfect verb (masc.))&  & & \\\cline{2-2}\cline{4-5}
 & 
Combination of the morphemes: \<ب> (present tense)
&  & REQUIRE+\<بت> & (she/it) requires \\
 & 
and \<ت> (3rd person imperfect verb (fem.))
&  & &  \\\hline
\<بن> & 
Combination of the morphemes: \<ب> (present tense) and \<ن>
& 10 & TARGET+\<بن> & (we) target \\\hline
\<فال> & Combination of the morphemes: \<ف> and \<ال> & 6 & TEAM+\<فال> & so the team \\\hline
\<هي>& 
Combination of the morphemes: \<ه> and \<ي> & 6 & REACT+\<هي> & 
(he/it) will react \\\hline
\<هت> & 
Combination of the morphemes: \<ه> and \<ت>
& 6 & AFFECT+\<هت> & 
(she/it) will affect \\\hline
\<كال> 
& Combination of the morphemes: \<ك> and \<ال> & 2 & WORKING LIFE+\<كال> & as (the) working life \\\hline
\<فب>& 
Combination of the morphemes: \<ف> and \<ب> (present tense)
& 2 & GROW+\<فب> & so (I) grow  \\\hline
\<هن>& 
Combination of the morphemes: \<ه> and \<ن>
& 2 & GUARANTEE+\<هن> & (we) will guarantee \\\hline
\<وا> + \<بي>& 
Combination of the morphemes: \<ب> (present tense) and \<وا> + \<ي> circumfix
& 2 & \<وا>\#target+\<بي> & (they) target\\\hline
\<ى> + \<بت>& 
Combination of the morphemes: \<ب> (present tense) and \<ى> + \<ت> circumfix
& 1 & \<ى>\#HANDLE+\<بت> & to handle\\\hline
\end{tabular}
\end{adjustbox}
\caption{Prefixes and suffixes occurring in ArzEn Intra-word CS.}
\label{table:arzen_affixes}
\end{table*}
